# Supplementary material for: Finding Bug-Inducing Program Environments
Source: arXiv:2304.10044 source file (2023-04-20)
Supplement: Supplementary file 1 [file appendix.tex]

\section{Appendix}
Tables \ref{tab:cov_analysis} and \ref{tab:cov_analysis2} show the total number of source files, along with the name of source files whose average line coverage is improved by at least 1\% by \afc for \texttt{Dnsmasq}, \texttt{Openssh}, \texttt{Openssl} and \texttt{Kamailio} subjects. The files which are directly environment related are shown by a (\checkmark). We can see that along with directly environment related codes, lots of indirectly environment-dependent source files are also covered by \afc.

\begin{table}[]
    \centering
    \caption{Qualitative analysis of coverage by \afc for Dnsmasq, Openssh and Openssl. (\checkmark: environment critical source codes)}
    \label{tab:cov_analysis}
    \begin{tabular}{p{.9cm}|c|p{3.1cm}|p{1cm}|p{1cm}}
    \textbf{Subject} & \textbf{\#f}     & \textbf{Source file} & \textbf{CHAOS (Lines\%)} & \textbf{\aflnet (Lines\%)}   \\\hline
     Dnsmasq & 40 & \checkmark cache.c & 23.6 & 6.3 \\
             & & dhcp-common.c & 25.1 & 2.1 \\
             & & dhcp.c & 6.7 & 0\\
             & & dhcp6.c & 13.6 & 0 \\
             & & \checkmark dnsmasq.c & 54.5 & 39.4 \\
             & & domain.c & 12.6 & 0 \\
             & & lease.c & 17.2 & 2.2 \\
             & & log.c & 62.0 & 50.8\\
             & & netlink.c & 56.2 & 46.2 \\
             & & \checkmark network.c & 51.8 & 26.8 \\
             & & option.c & 58.8 & 11.7 \\
             & & radv.c & 12.0 & 0 \\
             & & rfc1035.c & 18.5 & 17.3 \\
             & & slaac.c & 9.9 & 0\\
             & & \checkmark util.c & 74.9 & 30.1 \\\hline
     Openssh & 381 & atomicio.c & 31.3 & 26.9 \\
             & & dispatch.c & 93.3 & 91.7 \\
             & & fmt\_scaled.c & 14.2 & 0 \\
             & & log.c & 46.2 & 44.6 \\
             & & \checkmark servconf.c & 43.1 & 32.3 \\
             & & session.c & 33 & 30.6  \\
             & & ssherr.c & 24.6 & 22.8 \\
             & & sshpty.c & 64.1 & 41.6 \\\hline
     Openssl & 1610 & crypto\slash ...\slash a\_bitstr.c & 40.2 & 35.2 \\
             & & crypto\slash ...\slash a\_mbstr.c & 48.9 & 47.4 \\
             & & crypto\slash a\_object.c & 28.6 & 10.1 \\
             & & crypto\slash a\_time.c & 34.4 & 0.3 \\
             & & crypto\slash a\_type.c & 16.2 & 11.8 \\
             & & crypto\slash a\_utf8.c & 23.3 & 12.0 \\
             & & crypto\slash asnl\_lib.c & 56.4 & 44.7 \\
             & & crypto\slash tasn\_dec.c & 65.5 & 49.1 \\
             & & crypto\slash tasn\_fre.c & 79.0& 76.4\\
             & & crypto\slash x\_info.c & 85.7 & 0 \\
             & & crypto\slash x\_pkey.c & 13.0 & 0 \\
             & & crypto\slash bsearch.c & 91.7 & 83.3 \\
             & & \checkmark crypto\slash buffer.c & 75.6 & 73.3 \\
             & & \checkmark crypto\slash conf\_api.c & 79.8 & 2.7 \\
             & & \checkmark crypto\slash conf\_def.c & 5.7 & 60.0\\
             & & \checkmark crypto\slash conf\_lib.c & 17.6 & 7.0 \\
             & & \checkmark crypto\slash conf\_mode.c & 28.6 & 24.8 \\
             & & crypto\slash ctype.c & 83.3 &50.0\\
             & & crypto\slash err.c & 60.9 & 59.1 \\
             & & crypto\slash encode.c & 47.1 & 38.2 \\
             & & \checkmark crypto\slash evp\_pkey.c & 25.8 & 12.1 \\
             & & crypto\slash otime.c & 56.2 & 0 \\
             & & crypto\slash ...\slash obj\_dat.c & 26.5 & 15.2 \\
             & & crypto\slash ...\slash obj\_lib.c & 46.4 & 14.3 \\
             & & crypto\slash ...\slash obj\_xref.c & 29.7 & 28.4 \\
             & & \checkmark crypto\slash ...\slash pem\_info.c & 24.5 & 0 \\
             & & \checkmark crypto\slash ...\slash pem\_lib.c & 31.4 & 36.4 \\
             & & \checkmark crypto\slash ...\slash pem\_oth.c & 100 & 83.3 \\
             & & \checkmark crypto\slash ...\slash rsa\_ameth.c & 15.3 & 12.1\\
             & &  \checkmark crypto\slash ...\slash rsa\_asn1.c & 50.0 & 42.1 \\
             & &  \checkmark crypto\slash ...\slash rsa\_ossl.c & 26.1 & 24.0 \\
             & & crypto\slash $\sim$stack.c & 61.0  & 54.5 \\
             & & \checkmark crypto\slash ...\slash loader\_file.c & 34.0 & 32.7 \\
             & & \checkmark crypto\slash x509\slash by\_file.c & 26.3 & 16.5 \\
             & & crypto\slash x509\slash v3\_addr.c & 2.6 & 0 \\
             & & crypto\slash x509\slash v3\_asid.c & 4.2 & 0.4 \\
             & & crypto\slash x509\slash v3\_purp.c & 23.4 & 16.7 \\
             & & \checkmark crypto\slash ...\slash x509\_cmp.c & 21.8 & 12.7 \\
             & & \checkmark crypto\slash ...\slash x509\_lu.c & 38.1 & 25.2\\
             & & \checkmark crypto\slash ...\slash x509\_set.c & 39.0 & 22.0 \\
             & & \checkmark crypto\slash ...\slash x509\_trs.c & 11.3 & 0.0\\
             & & \checkmark crypto\slash ...\slash x509\_vfy.c & 22.2 & 12.2 \\
             & & crypto\slash x509\slash x\_name.c & 51.1 & 47.4 \\
             & & \checkmark crypto\slash x509\slash x\_pubkey.c & 18.3 & 14.1 \\
             & & \checkmark crypto\slash x509\slash x\_x509.c & 58.8 & 52.9 \\
             & & include\slash ...\slash bio.h & 100 & 0 \\
             & & \checkmark include\slash ...\slash conf.h & 100 & 50\\
             & & ssl\slash ssl\_rsa.c & 7 & 5.8 \\\hline
    \end{tabular}
\end{table}

\begin{table}[]
    \centering
    \caption{Qualitative analysis of coverage by \afc for Kamailio (\checkmark: environment critical source codes) }
    \label{tab:cov_analysis2}
    \begin{tabular}{p{.9cm}|c|p{3.1cm}|p{1cm}|p{1cm}}
    \textbf{Subject} & \textbf{\#f}     & \textbf{Source file} & \textbf{CHAOS (Lines\%)} & \textbf{\aflnet (Lines\%)}   \\\hline
         Kamailio & 2802 & \checkmark core\slash cfg.lex & 52.7 & 34.4\\
              & & \checkmark core\slash cfg.tab.c & 28.0 & 13.1\\ 
              & & \checkmark core\slash cfg.y & 34.8 & 18.5\\
              & & \checkmark core\slash cfg\slash cfg.c & 54.8 & 41.7\\
              & & \checkmark core\slash cfg\slash cfg\_script.c & 25.4 & 0\\
              & & core\slash ip\_addr.h & 35.5& 32.8 \\
              & & \checkmark core\slash lex.yy.c & 56.3 & 40.3 \\
             && core\slash modparam.c & 46.4 & 24.3 \\
             && core\slash counters.c & 52.9 & 51.8\\
             && core\slash daemonize.c & 10.2& 9.0\\
             && core\slash dprint.c & 17.9 & 16.8 \\
             && core\slash events.c & 24.3 & 22.8\\
             && core\slash flags.c & 31.2& 21.9\\
%              && core\slash parser\slash digest\_digest\_parser.c & 7.1 & 0 \\
              && \checkmark digest\_parser.c & 7.1 & 0 \\
%             && core\slash parser\slash parse\_addr\_spec.c & 82.4 & 79.0 \\
             && \checkmark parse\_addr\_spec.c & 82.4 & 79.0 \\
%              && core\slash parser\slash parse\_methods.c & 63.5 & 57.1 \\
              && \checkmark parse\_methods.c & 63.5 & 57.1 \\
%              && core\slash parser\slash parse\_nameaddr.c & 68.2 & 63.6 \\
              && \checkmark parse\_nameaddr.c & 68.2 & 63.6 \\
%              && core\slash parser\slash parse\_param.c & 25.6 & 19.1 \\
              && \checkmark parse\_param.c & 25.6 & 19.1 \\
              && \checkmark core\slash ppcfg.c & 24.8 & 20.0 \\
              && core\slash pt.c & 23.7 & 14.2 \\
              && core\slash pvapi.c & 46.7 & 42.5 \\
              && core\slash resolve.h & 100 & 50\\
              && core\slash rvalue.c & 21.2 & 17.6  \\
              && \checkmark core\slash socket\_info.c & 26.0 & 21.7 \\
              & & core\slash sr\_module.c &46.9 & 41.9 \\
              && \checkmark core\slash timer\_proc.c & 13.1 & 7.2 \\
              & & core\slash user\_avp.c & 12.6 &11.5 \\
              & & \checkmark lib\slash srdb1\slash db.c & 9.8 & 0 \\
              & & \checkmark main.c & 30.4 & 28.5\\
%              & & modules\slash auth\slash auth\_mode.c & 8.6 & 0\\
              & & auth\_mode.c & 8.6 & 0\\
%              & & modules\slash auth\slash nc.c & 3.8 & 0\\
%              & & modules\slash auth\slash nid.c & 11.5 & 0\\
%              & & modules\slash auth\slash ot\_nonce.c & 4.2 & 0\\
%              & & modules\slash auth\slash sl.h & 55.6 & 0\\
%              & & modules\slash auth\_db\slash auth\_db\_mode.c & 7.1 & 0\\
%              & & modules\slash debugger\slash debugger\_api.c & 6.1 & 0\\
%              & & modules\slash debugger\slash debugger\_mode.c & 11.0 & 0\\
%              & & modules\slash nethelper\slash nethelper.c & 4.6 & 0\\
%              & & modules\slash nethelper\slash sip\_pinger.h & 8.7 & 0\\
%              & & modules\slash nethelper\slash ut.h & 13.2 & 0\\
%              & & modules\slash permissions\slash address.c & 3.0 & 0\\
%              & & modules\slash permissions\slash permissions.c & 2.1 & 0\\
%              & & modules\slash permissions\slash trusted.c & 1.5 & 0\\
%              & & modules\slash pv\slash pv\_svar.c & 17.6 & 16.3\\
%              & & modules\slash rtpproxy\slash rtpproxy.c & 14.3 & 0\\
%              & & modules\slash rtpproxy\slash tm\_load.h & 62.5 & 0\\
%              & & modules\slash rtpproxy\slash ut.h & 16.4 & 0\\
%              & & modules\slash usrloc\slash ul\_callback.c & 29.7 & 27.0
              & & auth\slash nc.c & 3.8 & 0\\
              & & auth\slash nid.c & 11.5 & 0\\
              & & auth\slash ot\_nonce.c & 4.2 & 0\\
              & & auth\slash sl.h & 55.6 & 0\\
              & & auth\_db\slash auth\_db\_mode.c & 7.1 & 0\\
              & & debugger\_api.c & 6.1 & 0\\
              & & debugger\_mode.c & 11.0 & 0\\
              & & nethelper\slash nethelper.c & 4.6 & 0\\
              & & nethelper\slash sip\_pinger.h & 8.7 & 0\\
              & & nethelper\slash ut.h & 13.2 & 0\\
              & & permissions\slash address.c & 3.0 & 0\\
              & & permissions\slash permissions.c & 2.1 & 0\\
              & & permissions\slash trusted.c & 1.5 & 0\\
              & & pv\slash pv\_svar.c & 17.6 & 16.3\\
              & & rtpproxy\slash rtpproxy.c & 14.3 & 0\\
              & & rtpproxy\slash tm\_load.h & 62.5 & 0\\
              & & rtpproxy\slash ut.h & 16.4 & 0\\
              & & usrloc\slash ul\_callback.c & 29.7 & 27.0
              \\\hline
%              PureFtpd & 135 & & &
    \end{tabular}
\end{table}
